# Supplementary material for: Algorithms for Efficient, Compact Online Data Stream Curation
Source: arXiv:2403.00266 source file (2024-03-01)
Supplement: Supplementary file 1 [file supplement.tex]

% \pragmaonce

% adapted from https://www.overleaf.com/learn/latex/Commands
\providecommand{\dissertationexclude}[1]{%
% adapted from https://tex.stackexchange.com/a/33577
\ifdefined\DISSERTATION
\else
#1
\fi
}

% \pragmaonce

% adapted from https://www.overleaf.com/learn/latex/Commands

\dissertationexclude{\section{Supplemental Material}}
\section{Memory Footprint Outcomes} \label{sec:memory_footprint_outcomes}

% \pragmaonce
% ^adapted from https://tex.stackexchange.com/a/195173

% adapted from https://tex.stackexchange.com/a/118450
\providecommand{
\def\dataname{}\def\fulldataname{}% \input{lib/importpath.tex}
\makeatletter
  \def\importpathx{\import@path}
\makeatother

\begin{table}

\begin{tabularx}{\columnwidth}{X | X | X | X | X | X}%
  \adjustbox{
    minipage=12em,
    rotate=90,
  }{
    \raggedright
    \bfseries
    Target Per-Column Memory Footprint (bits)
    \par
  }
  & \adjustbox{
      minipage=12em,
      rotate=90,
    }{
      \raggedright
      \bfseries
      Actual Mean Per-Column Memory Footprint (bits)
      \par
  }
  & \adjustbox{
      minipage=12em,
      rotate=90,
    }{
      \raggedright
      \bfseries
      Memory Footprint Percent Error
      \par
  }
  & \adjustbox{
      minipage=12em,
      rotate=90,
    }{
      \raggedright
      \bfseries
      Fingerprint Differentia Width (bits)
      \par
  }
  & \adjustbox{
      minipage=12em,
      rotate=90,
    }{
      \raggedright
      \bfseries
      Stratum Retention Policy
      \par
  }
  & \adjustbox{
      minipage=12em,
      rotate=90,
    }{
      \raggedright
      \bfseries
      Retention Policy Resolution Parameter
      \par
  }
  \\\hline\hline  % specify table head
  \csvreader[
    filter expr={
          test{\ifnumgreater{\thecsvinputline}{2}}
    }
  ]{\importpathx submodules/hereditary-stratigraph-concept/binder/phylogenetic-inference/\fulldataname }{}% use head of csv as column names
{
  \csvcolix
  & \num[round-precision=1,round-mode=places]{\csvcolii}
  &
  \ifthenelse{
    \lengthtest{\csuse{csvcolii}pt > \csuse{csvcolix}pt}
    }{\cellcolor{red!25}}{}%

  \num[round-precision=1,round-mode=places]{
    \fpeval{ 100 * \csvcolii / \csvcolix - 100 }
  }
  & \csvcolvi
  &
  \StrDel{\csvcolvii}{a}[\temp]
  \StrDel{\temp}{b}[\temp]
  \StrDel{\temp}{c}[\temp]
  \StrDel{\temp}{d}[\temp]
  \StrDel{\temp}{e}[\temp]
  \StrDel{\temp}{f}[\temp]
  \StrDel{\temp}{g}[\temp]
  \StrDel{\temp}{h}[\temp]
  \StrDel{\temp}{i}[\temp]
  \StrDel{\temp}{j}[\temp]
  \StrDel{\temp}{k}[\temp]
  \StrDel{\temp}{l}[\temp]
  \StrDel{\temp}{m}[\temp]
  \StrDel{\temp}{n}[\temp]
  \StrDel{\temp}{o}[\temp]
  \StrDel{\temp}{p}[\temp]
  \StrDel{\temp}{q}[\temp]
  \StrDel{\temp}{r}[\temp]
  \StrDel{\temp}{s}[\temp]
  \StrDel{\temp}{t}[\temp]
  \StrDel{\temp}{u}[\temp]
  \StrDel{\temp}{v}[\temp]
  \StrDel{\temp}{w}[\temp]
  \StrDel{\temp}{x}[\temp]
  \StrDel{\temp}{y}[\temp]
  \StrDel{\temp}{z}
  & \csvcolviii
  \\
}% specify your columns here
\end{tabularx}
\caption{
Hereditary stratigraph column memory footprint outcomes for phylogenetic reconstruction experiments on the \dataname dataset.
All treatments' stratum retention policies were parameterized to use as much of the target per-column memory footprint as possible without exceeding it.
Treatments where the stratum retention policy could not be parameterized low enough to meet the target per-column memory footprint are highlighted in red.
TDPR denotes the ``Tapered Depth-Proportional Resolution'' policy and RPR denotes the ``Recency-Proportional Resolution'' policy.
}

% adapted from https://tex.stackexchange.com/a/15708
\StrSubstitute{\dataname}{ }{-}[\temp]
\StrSubstitute{\temp}{A}{a}[\temp]
\StrSubstitute{\temp}{B}{b}[\temp]
\StrSubstitute{\temp}{C}{c}[\temp]
\StrSubstitute{\temp}{D}{d}[\temp]
\StrSubstitute{\temp}{E}{e}[\temp]
\StrSubstitute{\temp}{F}{f}[\temp]
\StrSubstitute{\temp}{G}{g}[\temp]
\StrSubstitute{\temp}{H}{h}[\temp]
\StrSubstitute{\temp}{I}{i}[\temp]
\StrSubstitute{\temp}{J}{j}[\temp]
\StrSubstitute{\temp}{K}{k}[\temp]
\StrSubstitute{\temp}{L}{l}[\temp]
\StrSubstitute{\temp}{M}{m}[\temp]
\StrSubstitute{\temp}{N}{n}[\temp]
\StrSubstitute{\temp}{O}{o}[\temp]
\StrSubstitute{\temp}{P}{p}[\temp]
\StrSubstitute{\temp}{Q}{q}[\temp]
\StrSubstitute{\temp}{R}{r}[\temp]
\StrSubstitute{\temp}{S}{s}[\temp]
\StrSubstitute{\temp}{T}{t}[\temp]
\StrSubstitute{\temp}{U}{u}[\temp]
\StrSubstitute{\temp}{V}{v}[\temp]
\StrSubstitute{\temp}{w}{w}[\temp]
\StrSubstitute{\temp}{X}{x}[\temp]
\StrSubstitute{\temp}{Y}{y}[\temp]
\StrSubstitute{\temp}{Z}{z}[\temp]

\def\labeltext{%
  {tab:experiment-column-sizes-\temp}%
}
\expandafter\label\labeltext
\end{table}

}[2]{
\def\dataname{#1}\def\fulldataname{#2}% \input{lib/importpath.tex}
\makeatletter
  \def\importpathx{\import@path}
\makeatother

\begin{table}

\begin{tabularx}{\columnwidth}{X | X | X | X | X | X}%
  \adjustbox{
    minipage=12em,
    rotate=90,
  }{
    \raggedright
    \bfseries
    Target Per-Column Memory Footprint (bits)
    \par
  }
  & \adjustbox{
      minipage=12em,
      rotate=90,
    }{
      \raggedright
      \bfseries
      Actual Mean Per-Column Memory Footprint (bits)
      \par
  }
  & \adjustbox{
      minipage=12em,
      rotate=90,
    }{
      \raggedright
      \bfseries
      Memory Footprint Percent Error
      \par
  }
  & \adjustbox{
      minipage=12em,
      rotate=90,
    }{
      \raggedright
      \bfseries
      Fingerprint Differentia Width (bits)
      \par
  }
  & \adjustbox{
      minipage=12em,
      rotate=90,
    }{
      \raggedright
      \bfseries
      Stratum Retention Policy
      \par
  }
  & \adjustbox{
      minipage=12em,
      rotate=90,
    }{
      \raggedright
      \bfseries
      Retention Policy Resolution Parameter
      \par
  }
  \\\hline\hline  % specify table head
  \csvreader[
    filter expr={
          test{\ifnumgreater{\thecsvinputline}{2}}
    }
  ]{\importpathx submodules/hereditary-stratigraph-concept/binder/phylogenetic-inference/\fulldataname }{}% use head of csv as column names
{
  \csvcolix
  & \num[round-precision=1,round-mode=places]{\csvcolii}
  &
  \ifthenelse{
    \lengthtest{\csuse{csvcolii}pt > \csuse{csvcolix}pt}
    }{\cellcolor{red!25}}{}%

  \num[round-precision=1,round-mode=places]{
    \fpeval{ 100 * \csvcolii / \csvcolix - 100 }
  }
  & \csvcolvi
  &
  \StrDel{\csvcolvii}{a}[\temp]
  \StrDel{\temp}{b}[\temp]
  \StrDel{\temp}{c}[\temp]
  \StrDel{\temp}{d}[\temp]
  \StrDel{\temp}{e}[\temp]
  \StrDel{\temp}{f}[\temp]
  \StrDel{\temp}{g}[\temp]
  \StrDel{\temp}{h}[\temp]
  \StrDel{\temp}{i}[\temp]
  \StrDel{\temp}{j}[\temp]
  \StrDel{\temp}{k}[\temp]
  \StrDel{\temp}{l}[\temp]
  \StrDel{\temp}{m}[\temp]
  \StrDel{\temp}{n}[\temp]
  \StrDel{\temp}{o}[\temp]
  \StrDel{\temp}{p}[\temp]
  \StrDel{\temp}{q}[\temp]
  \StrDel{\temp}{r}[\temp]
  \StrDel{\temp}{s}[\temp]
  \StrDel{\temp}{t}[\temp]
  \StrDel{\temp}{u}[\temp]
  \StrDel{\temp}{v}[\temp]
  \StrDel{\temp}{w}[\temp]
  \StrDel{\temp}{x}[\temp]
  \StrDel{\temp}{y}[\temp]
  \StrDel{\temp}{z}
  & \csvcolviii
  \\
}% specify your columns here
\end{tabularx}
\caption{
Hereditary stratigraph column memory footprint outcomes for phylogenetic reconstruction experiments on the \dataname dataset.
All treatments' stratum retention policies were parameterized to use as much of the target per-column memory footprint as possible without exceeding it.
Treatments where the stratum retention policy could not be parameterized low enough to meet the target per-column memory footprint are highlighted in red.
TDPR denotes the ``Tapered Depth-Proportional Resolution'' policy and RPR denotes the ``Recency-Proportional Resolution'' policy.
}

% adapted from https://tex.stackexchange.com/a/15708
\StrSubstitute{\dataname}{ }{-}[\temp]
\StrSubstitute{\temp}{A}{a}[\temp]
\StrSubstitute{\temp}{B}{b}[\temp]
\StrSubstitute{\temp}{C}{c}[\temp]
\StrSubstitute{\temp}{D}{d}[\temp]
\StrSubstitute{\temp}{E}{e}[\temp]
\StrSubstitute{\temp}{F}{f}[\temp]
\StrSubstitute{\temp}{G}{g}[\temp]
\StrSubstitute{\temp}{H}{h}[\temp]
\StrSubstitute{\temp}{I}{i}[\temp]
\StrSubstitute{\temp}{J}{j}[\temp]
\StrSubstitute{\temp}{K}{k}[\temp]
\StrSubstitute{\temp}{L}{l}[\temp]
\StrSubstitute{\temp}{M}{m}[\temp]
\StrSubstitute{\temp}{N}{n}[\temp]
\StrSubstitute{\temp}{O}{o}[\temp]
\StrSubstitute{\temp}{P}{p}[\temp]
\StrSubstitute{\temp}{Q}{q}[\temp]
\StrSubstitute{\temp}{R}{r}[\temp]
\StrSubstitute{\temp}{S}{s}[\temp]
\StrSubstitute{\temp}{T}{t}[\temp]
\StrSubstitute{\temp}{U}{u}[\temp]
\StrSubstitute{\temp}{V}{v}[\temp]
\StrSubstitute{\temp}{w}{w}[\temp]
\StrSubstitute{\temp}{X}{x}[\temp]
\StrSubstitute{\temp}{Y}{y}[\temp]
\StrSubstitute{\temp}{Z}{z}[\temp]

\def\labeltext{%
  {tab:experiment-column-sizes-\temp}%
}
\expandafter\label\labeltext
\end{table}

}

\def\dataname{NK EcoEA Selection}\def\fulldataname{a=actual_retained_bits+source=nk_ecoeaselection_seed110_pop100_mut.01_snapshot_3000.csv}

\def\dataname{NK Lexicase Selection}\def\fulldataname{a=actual_retained_bits+source=nk_lexicaseselection_seed110_pop165_mut.01_snapshot_500.csv}

\def\dataname{NK Random Selection}\def\fulldataname{a=actual_retained_bits+source=nk_randomselection_seed7_pop100_mut.01_snapshot_5000.csv}

\def\dataname{NK Sharing Selection}\def\fulldataname{a=actual_retained_bits+source=nk_sharingselection_seed10_pop100_mut.01_snapshot_5000.csv}

\def\dataname{NK Tournament Selection}\def\fulldataname{a=actual_retained_bits+source=nk_tournamentselection_seed140_pop100_mut.01_snapshot_5000.csv}

\section{Differentia Size} \label{sec:differentia-size-full}

\section{Retention Policy} \label{sec:retention-policy-full}

\section{Condemner Implementations}
\label{sec:condemner-implementations}

% \pragmaonce

% adapted from https://www.overleaf.com/learn/latex/Commands
\providecommand{\dissertationelse}[2]{%
% adapted from https://tex.stackexchange.com/a/33577
\ifdefined\DISSERTATION
#1
\else
#2
\fi
}

\provideenvironment{lstinputlistinghandle}{}{}

{\makeatletter\if@twocolumn\onecolumn\fi\makeatother
\begin{lstinputlistinghandle}
\lstinputlisting[%
language=Python,
caption={
  Depth-proportional resolution policy condemner implementation.
},
label={lst:StratumRetentionCondemnerDepthProportionalResolution},
style=mypython,
basicstyle=\dissertationelse{\fontsize{9}{10}\selectfont}{\scriptsize},
]{submodules/hstrat/hstrat/hstrat/stratum_retention_condemners/StratumRetentionCondemnerDepthProportionalResolution.py}
\end{lstinputlistinghandle}
}

\provideenvironment{lstinputlistinghandle}{}{}

{\makeatletter\if@twocolumn\onecolumn\fi\makeatother
\begin{lstinputlistinghandle}
\lstinputlisting[%
language=Python,
caption={
  Fixed resolution policy condemner implementation.
},
label={lst:StratumRetentionCondemnerFixedResolution},
style=mypython,
basicstyle=\dissertationelse{\fontsize{9}{10}\selectfont}{\scriptsize},
]{submodules/hstrat/hstrat/hstrat/stratum_retention_condemners/StratumRetentionCondemnerFixedResolution.py}
\end{lstinputlistinghandle}
}

\provideenvironment{lstinputlistinghandle}{}{}

{\makeatletter\if@twocolumn\onecolumn\fi\makeatother
\begin{lstinputlistinghandle}
\lstinputlisting[%
language=Python,
caption={
  MRCA-recency-proportional resolution policy condemner implementation.
},
label={lst:StratumRetentionCondemnerRecencyProportionalResolution},
style=mypython,
basicstyle=\dissertationelse{\fontsize{9}{10}\selectfont}{\scriptsize},
]{submodules/hstrat/hstrat/hstrat/stratum_retention_condemners/StratumRetentionCondemnerRecencyProportionalResolution.py}
\end{lstinputlistinghandle}
}

\provideenvironment{lstinputlistinghandle}{}{}

{\makeatletter\if@twocolumn\onecolumn\fi\makeatother
\begin{lstinputlistinghandle}
\lstinputlisting[%
language=Python,
caption={
  Tapered depth-proportional resolution policy condemner implementation.
},
label={lst:StratumRetentionCondemnerTaperedDepthProportionalResolution},
style=mypython,
basicstyle=\dissertationelse{\fontsize{9}{10}\selectfont}{\scriptsize},
]{submodules/hstrat/hstrat/hstrat/stratum_retention_condemners/StratumRetentionCondemnerTaperedDepthProportionalResolution.py}
\end{lstinputlistinghandle}
}

\section{Predicate Implementations}
\label{sec:predicate-implementations}

\provideenvironment{lstinputlistinghandle}{}{}

{\makeatletter\if@twocolumn\onecolumn\fi\makeatother
\begin{lstinputlistinghandle}
\lstinputlisting[%
language=Python,
caption={
  Depth-proportional resolution policy predicate implementation, including method to calculate exact number of strata retained by generation and method to calculate stratum deposition rank from column index.
},
label={lst:StratumRetentionPredicateDepthProportionalResolution},
style=mypython,
basicstyle=\dissertationelse{\fontsize{9}{10}\selectfont}{\scriptsize},
]{submodules/hstrat/hstrat/hstrat/stratum_retention_predicates/StratumRetentionPredicateDepthProportionalResolution.py}
\end{lstinputlistinghandle}
}

\provideenvironment{lstinputlistinghandle}{}{}

{\makeatletter\if@twocolumn\onecolumn\fi\makeatother
\begin{lstinputlistinghandle}
\lstinputlisting[%
language=Python,
caption={
  Fixed resolution policy predicate implementation, including method to calculate exact number of strata retained by generation and method to calculate stratum deposition rank from column index.
},
label={lst:StratumRetentionPredicateFixedResolution},
style=mypython,
basicstyle=\dissertationelse{\fontsize{9}{10}\selectfont}{\scriptsize},
]{submodules/hstrat/hstrat/hstrat/stratum_retention_predicates/StratumRetentionPredicateFixedResolution.py}
\end{lstinputlistinghandle}
}

\provideenvironment{lstinputlistinghandle}{}{}

{\makeatletter\if@twocolumn\onecolumn\fi\makeatother
\begin{lstinputlistinghandle}
\lstinputlisting[%
language=Python,
caption={
  MRCA-recency-proportional resolution policy predicate implementation, including method to calculate exact number of strata retained by generation and method to calculate stratum deposition rank from column index.
},
label={lst:StratumRetentionPredicateRecencyProportionalResolution},
style=mypython,
basicstyle=\dissertationelse{\fontsize{9}{10}\selectfont}{\scriptsize},
]{submodules/hstrat/hstrat/hstrat/stratum_retention_predicates/StratumRetentionPredicateRecencyProportionalResolution.py}
\end{lstinputlistinghandle}
}

\provideenvironment{lstinputlistinghandle}{}{}

{\makeatletter\if@twocolumn\onecolumn\fi\makeatother
\begin{lstinputlistinghandle}
\lstinputlisting[%
language=Python,
caption={
  Tapered depth-proportional resolution policy predicate implementation, including method to calculate exact number of strata retained by generation and method to calculate stratum deposition rank from column index.
},
label={lst:StratumRetentionPredicateTaperedDepthProportionalResolution},
style=mypython,
basicstyle=\dissertationelse{\fontsize{9}{10}\selectfont}{\scriptsize},
]{submodules/hstrat/hstrat/hstrat/stratum_retention_predicates/StratumRetentionPredicateTaperedDepthProportionalResolution.py}
\end{lstinputlistinghandle}
}

\section{Miscellaneous} \label{sec:hstrat-miscellaneous}

\begin{sidewaystable}[]
\begin{tabular}{lllll}
Selection Scheme & Per-bit Mutation Rate & Number Generations & Population Size & Phylogeny Download URL \\
Eco-EA           & 0.01                  & 3000               & 100             & \url{https://osf.io/5d3be/} \\
Lexicase         & 0.01                  & 500                & 165             & \url{https://osf.io/8ycq7/} \\
Random           & 0.01                  & 5000               & 100             & \url{https://osf.io/ydxt7/} \\
Sharing          & 0.01                  & 5000               & 100             & \url{https://osf.io/cz9fk/} \\
Tournament       & 0.01                  & 5000               & 100             & \url{https://osf.io/5ubn8/}
\end{tabular}
\caption{
Evolutionary conditions of ground-truth phylogenies taken from \citep{dolson2018applying}.
} \label{tab:ground-truth-phylogenies}
\end{sidewaystable}
