# Supplementary material for: Algorithms for Efficient, Compact Online Data Stream Curation
Source: arXiv:2403.00266 source file (2024-03-01)
Supplement: Supplementary file 2 [file differentia-size-full.tex]

{
\onecolumn
\section{Differentia Size} \label{sec:differentia-size-full}

\providecommand{\PreserveBackslash}[1]{\let\temp=\\#1\let\\=\temp}

% adapted from https://tex.stackexchange.com/a/449117
\newcolumntype{C}[1]{>{\PreserveBackslash\centering}p{#1}}

\csvreader[
  longtable=C{3cm}cccccc,
  table head=\caption{
    Comparison of phylogenetic reconstruction quality across differentia bit counts.
    Reconstruction quality measured as clustering information distance (lower is better), mutual clustering information (higher is better), and generalized Robinson-Foulds similarity (higher is better) between reconstructed phylogeny and ground truth phylogeny \citep{smith2020information, smith2020treedist}.
    RPR is recency-proportional resolution stratum retention policy and TDPR is tapered depth-proportional resolution stratum retention policy.
  }\label{tab:reconstruction-quality-results-by-differentia-bits} \\
    \toprule \thead{Tree Comparison Metric} & \thead{Selection\\ Scheme} & \thead{Stratum\\ Retention\\ Policy} & \thead{Target\\ Num\\ Column\\ Bits} & \thead{1 \\Differentia \\ Bit\\ Score} & \thead{8 \\Differentia \\ Bits\\ Score} & \thead{64 \\Differentia \\ Bits\\ Score} \\ \midrule\endhead
    \bottomrule\endfoot,
  late after line=\\,
]{%
submodules/hereditary-stratigraph-concept/binder/reconstruction-quality/outplots/reconstruction_quality_results_by_differentia_bits.csv%
}{}{%
\vcell{\csvcoli} & \vcell{\csvcolii} & \vcell{\csvcoliii} & \vcell{\csvcoliv} & \vcell{\csvcolv} & \vcell{\csvcolvi} & \vcell{\csvcolvii} \\[-\rowheight]
\printcellmiddle & \printcellmiddle & \printcellmiddle & \printcellmiddle & \printcellmiddle & \printcellmiddle & \printcellmiddle \\
}

\begin{sidewaysfigure}
  \includegraphics[width=\linewidth]{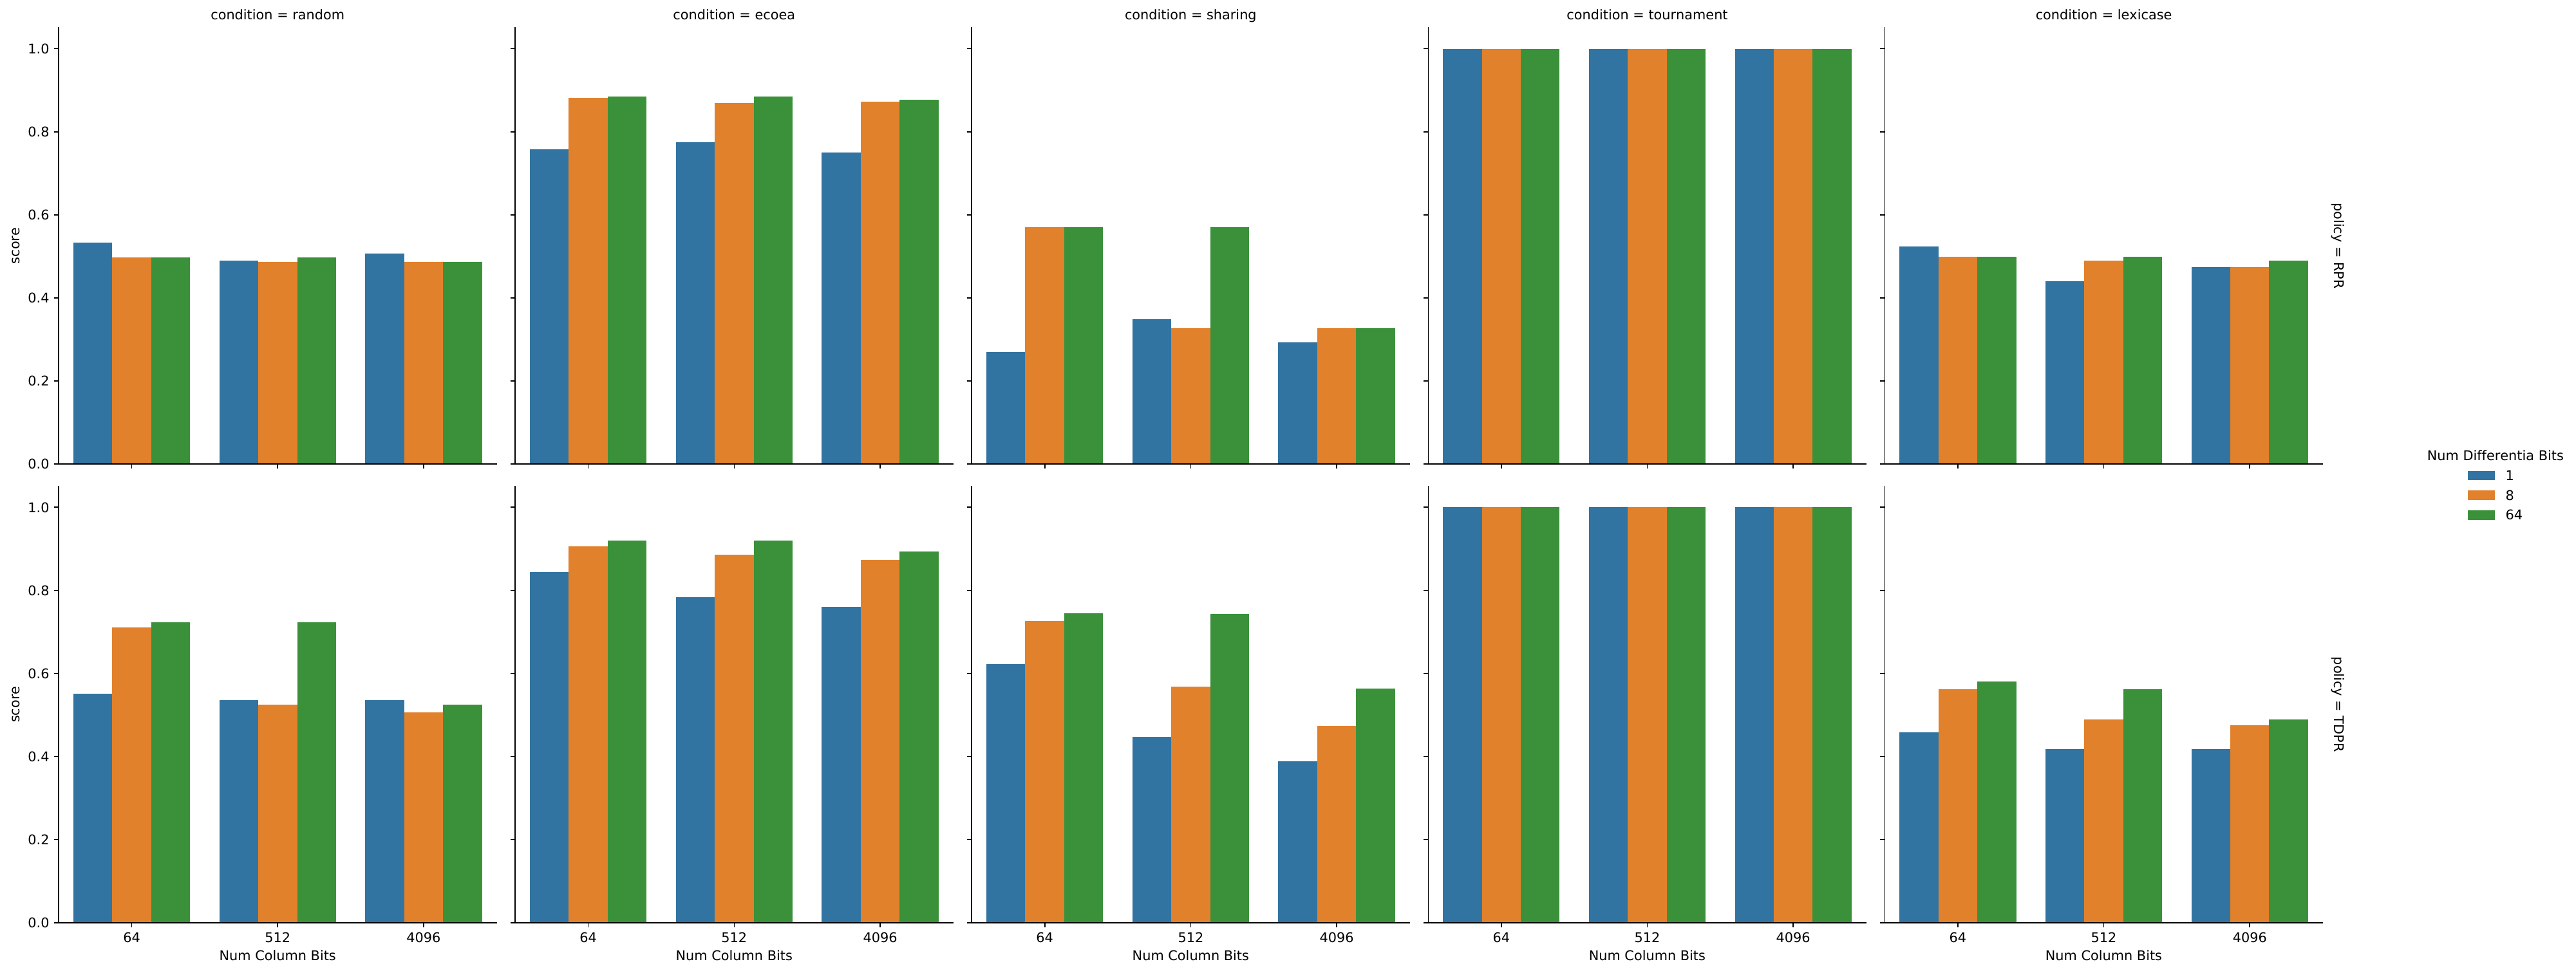}
  \caption{
  Comparison of phylogenetic reconstruction quality across differentia bit counts.
  Reconstruction quality measured as clustering information distance between reconstructed phylogeny and ground truth phylogeny \citep{smith2020information, smith2020treedist}.
  Lower is better.
  RPR is recency-proportional resolution stratum retention policy and TDPR is tapered depth-proportional resolution stratum retention policy.
  }
  \label{fig:diffbits-clustering-information-distance}
\end{sidewaysfigure}

\begin{sidewaysfigure}
  \includegraphics[width=\linewidth]{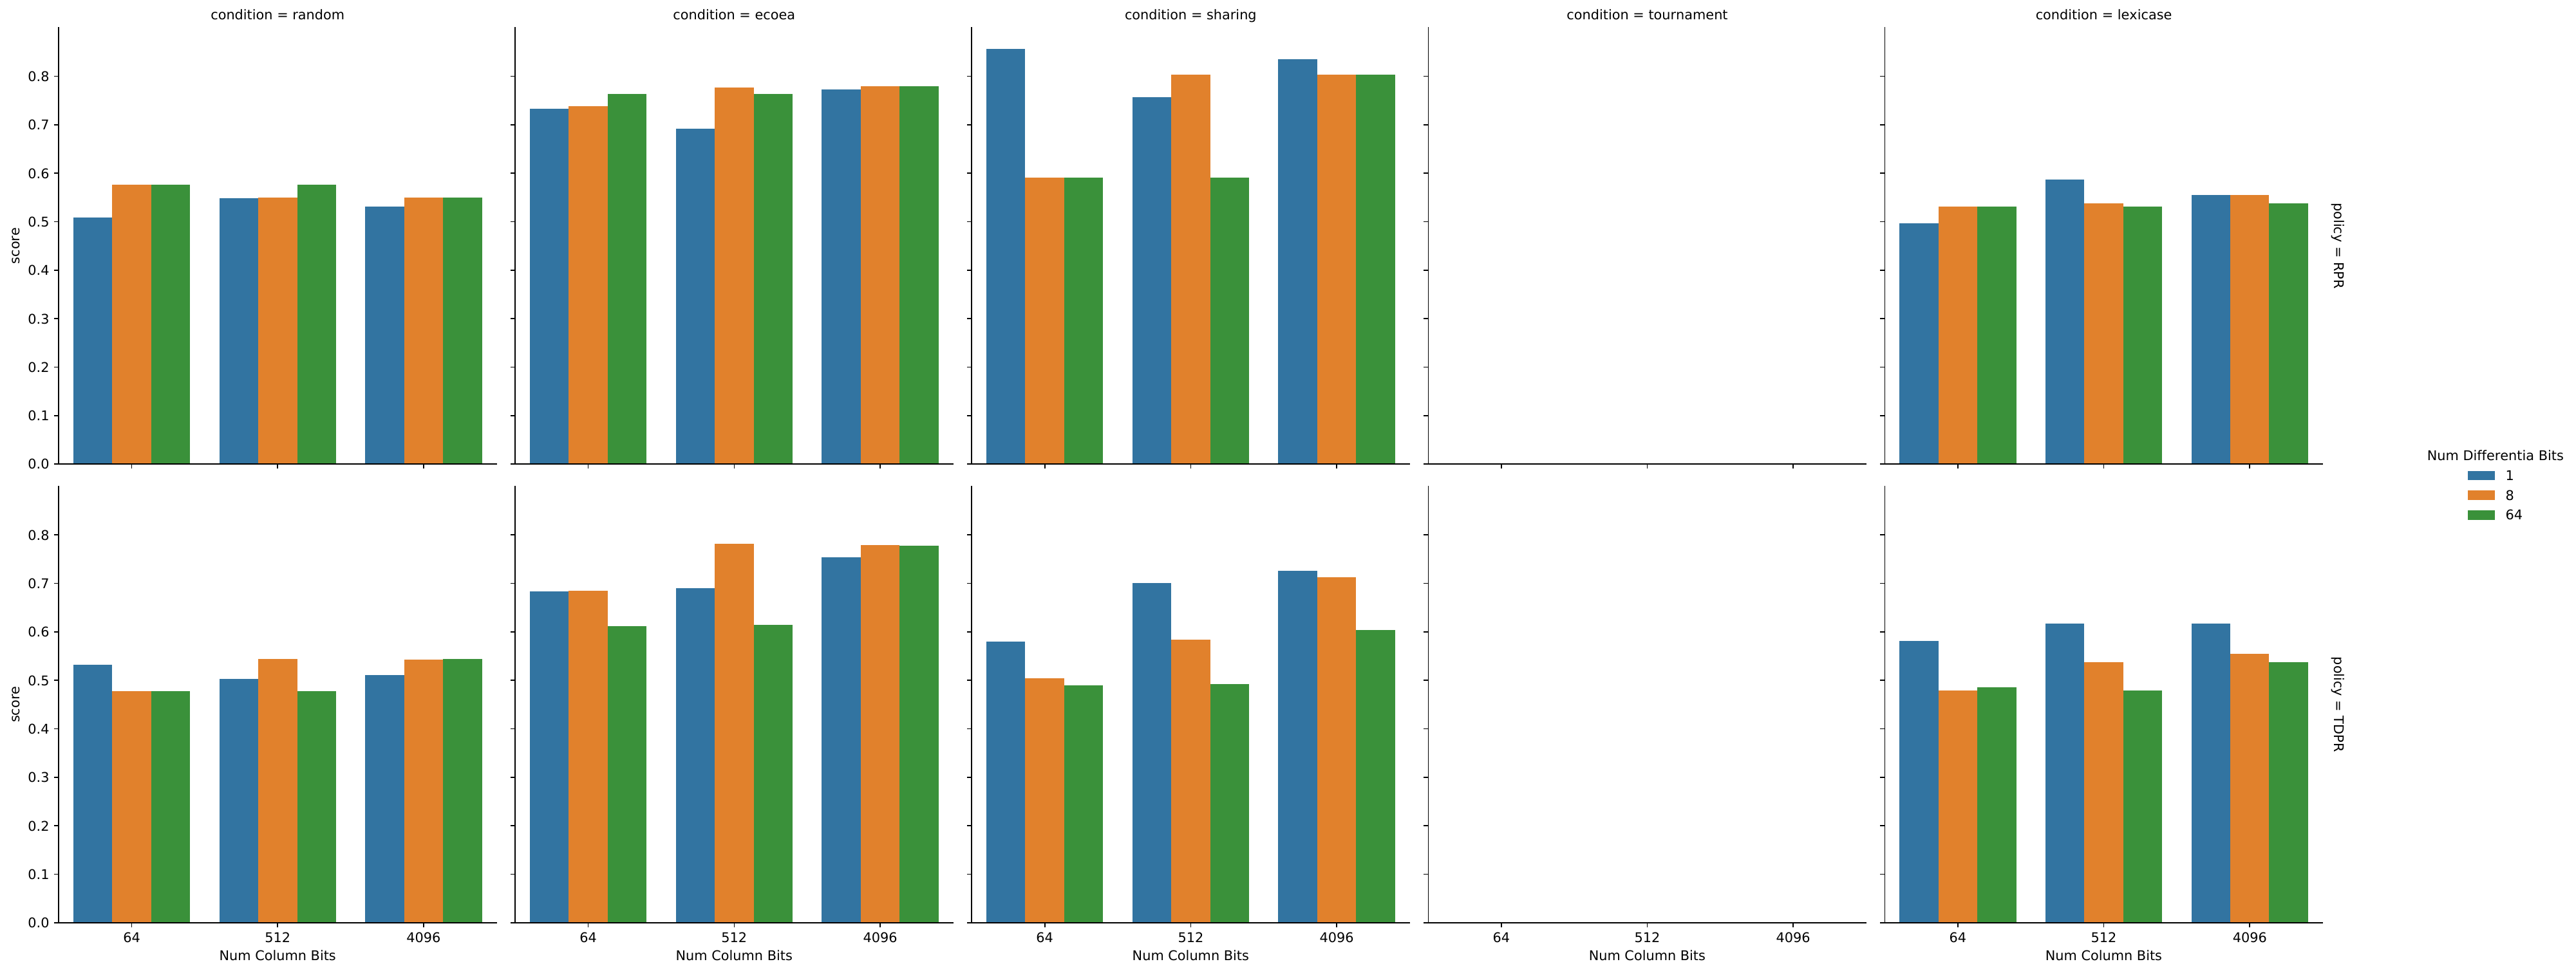}
  \caption{
  Comparison of phylogenetic reconstruction quality across differentia bit counts.
  Reconstruction quality measured as mutual clustering information between reconstructed phylogeny and ground truth phylogeny \citep{smith2020information, smith2020treedist}.
  Higher is better.
  RPR is recency-proportional resolution stratum retention policy and TDPR is tapered depth-proportional resolution stratum retention policy.
  }
  \label{fig:diffbits-mutual-clustering-information}
\end{sidewaysfigure}

\begin{sidewaysfigure}
  \includegraphics[width=\linewidth]{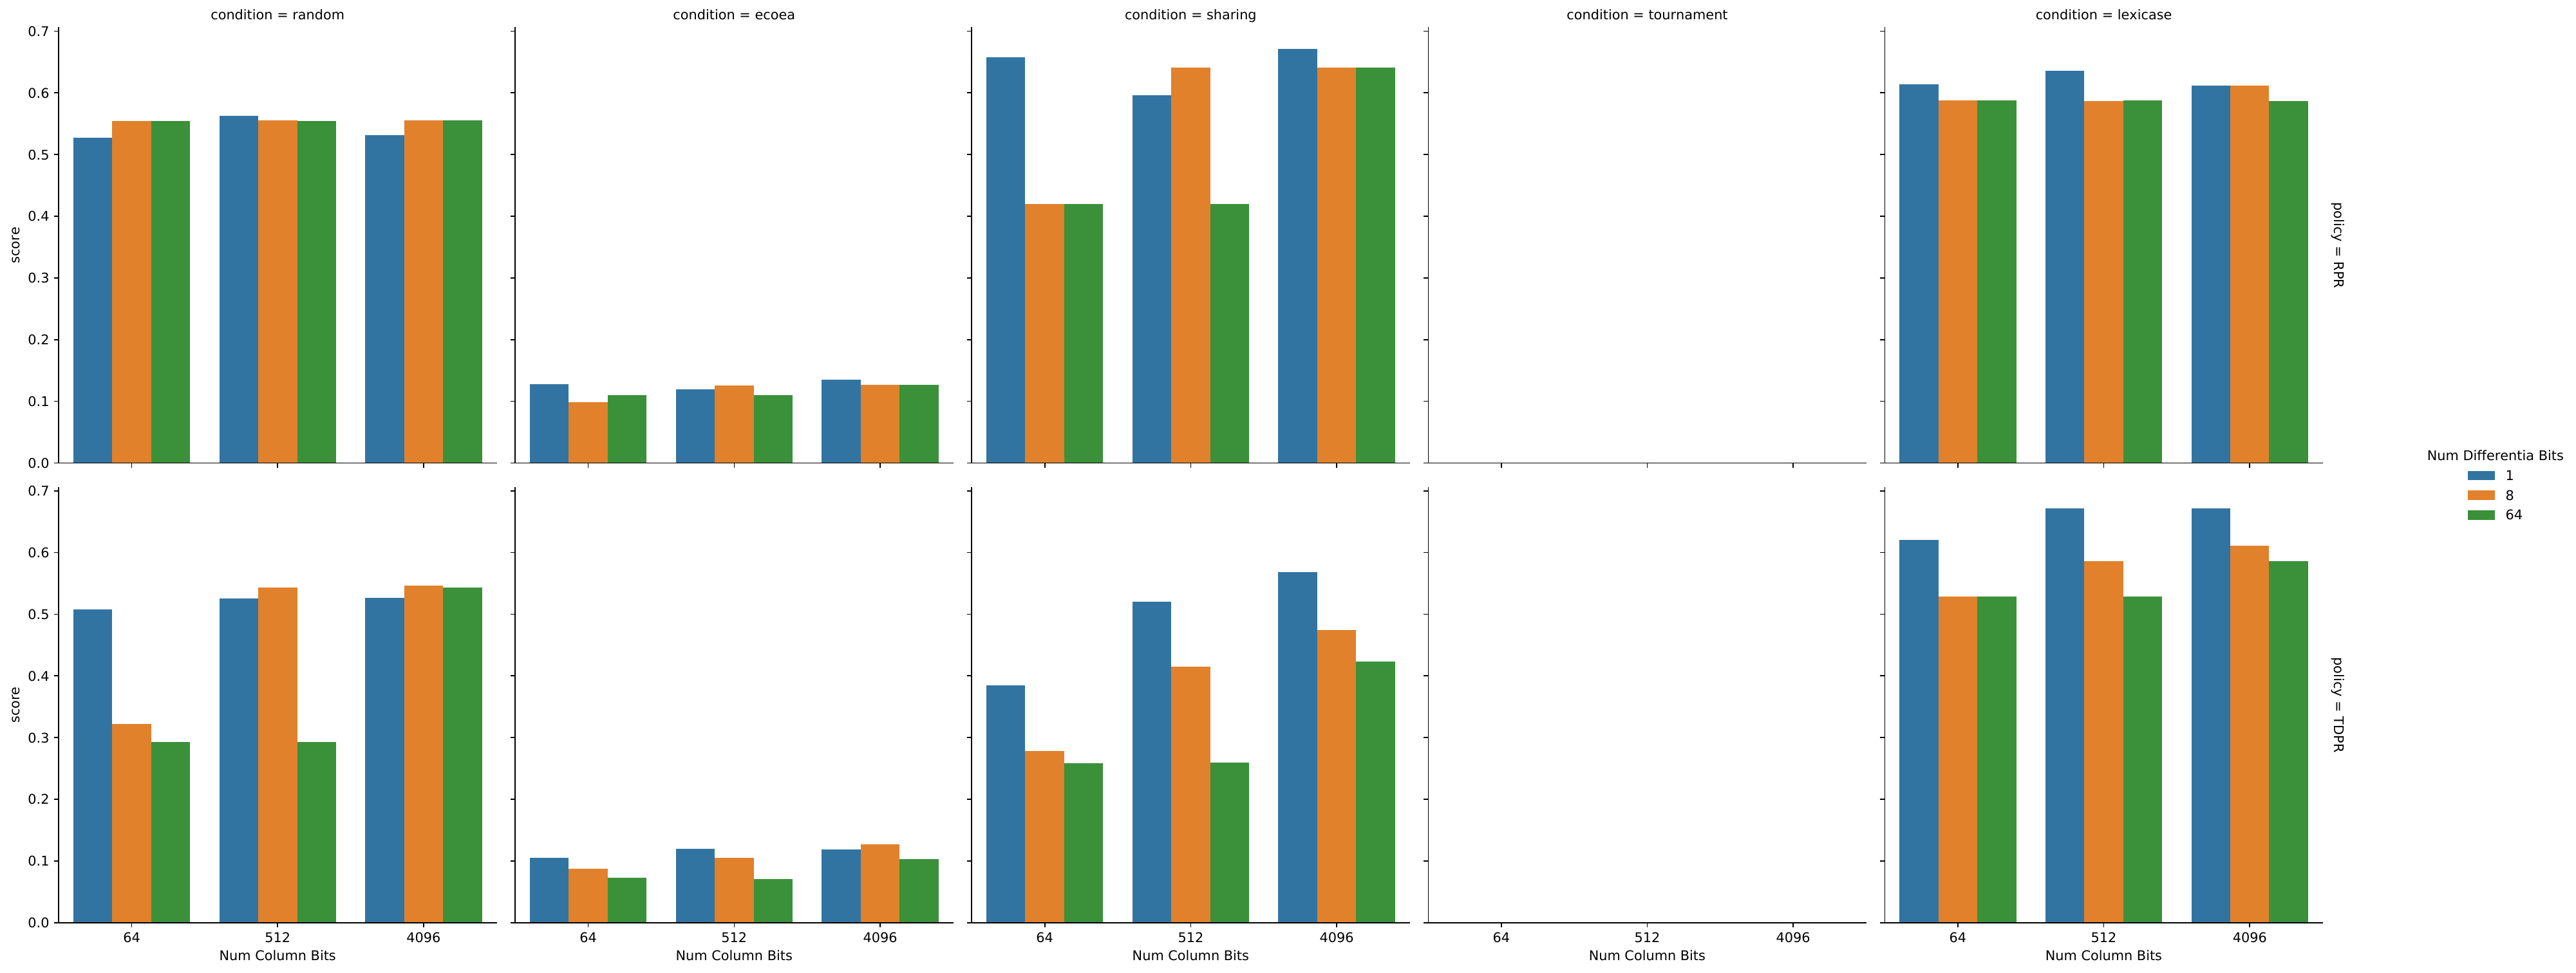}
  \caption{
  Comparison of phylogenetic reconstruction quality across differentia bit counts.
  Reconstruction quality measured as generalized Robinson-Foulds similarity between reconstructed phylogeny and ground truth phylogeny \citep{smith2020information, smith2020treedist}.
  Higher is better.
  RPR is recency-proportional resolution stratum retention policy and TDPR is tapered depth-proportional resolution stratum retention policy.
  }
  \label{fig:diffbits-robinson-foulds-similarity}
\end{sidewaysfigure}

}
