# Supplementary material for: Algorithms for Efficient, Compact Online Data Stream Curation
Source: arXiv:2403.00266 source file (2024-03-01)
Supplement: Supplementary file 4 [file perfect-tracking-space.tex]

\section{Additional notes on the memory requirements of perfect tracking} \label{sec:perfect-tracking-space-supp}
% TODO: section name that isn't monstorously long

Note that perfect phylogeny tracking algorithms are designed to plug into a larger computational process.
For phylogeny tracking to be relevant, this computational process must have a collection of $N$ objects that are currently eligilble to be copied (in evolutionary terms, the population).
Therefore, the space complexity of this process must be at least $\mathcal{O}(N)$.
As long as the expected size of $T$ scales no faster than $\mathcal{O}(N)$, then, phylogeny tracking will not be the primary factor determining memory usage.
While the memory cost of phylogeny tracking could still be significant in these cases, it is unlikely to be the primary factor determining whether running the program is tractable.

Previously, we noted that cases where perfect tracking with pruning achieves its worst case size order of growth are esoteric.
There are two ways that theses situations can occur:

\begin{itemize}
\item $N$ is continuously increasing.
\item There is effectively no coalescence.
\end{itemize}

In case 1, the space complexity of the external computational process will also be growing at least as fast as $\mathcal{O}(N)$.
Because $N$ itself is growing, this behavior should overwhelm the size of the history in $T$ in most cases.
Even in the (completely unrealistic) case where $N$ is allowed to reach infinity, there is an argument to be made that the internal nodes of $T$ would not be substantially contributing to memory complexity.
While this argument is beyond the scope of this paper, it would center around the fact that most evolutionarily-realistic coalescence proceses ``come down from infinity'' \citep{berestyckiRecentProgressCoalescent2009}.
% Indeed, unless $N$ starts out infinite, any process observed by phylogenetic tracking must come down from infinity, as they 

Case 2 is a legitimate circumstance where worst case memory complexity could occur. 
It would occur in cases where every member of the population has (approximately) one offspring.
While this level of regularity is unlikely in the context of evolution, it could happen when tracking non-evolutionry digital artifacts.
