# Supplementary material for: Algorithms for Efficient, Compact Online Data Stream Curation
Source: arXiv:2403.00266 source file (2024-03-01)
Supplement: Supplementary file 5 [file supplement.tex]

\section{Supplemental Materials}

\section{Example} \label{sec:example}

example \citep{gropp1996high}
