# Supplementary material for: Algorithms for Efficient, Compact Online Data Stream Curation
Source: arXiv:2403.00266 source file (2024-03-01)
Supplement: Supplementary file 8 [file condemner-implementations.tex]

\section{Condemner Implementations}
\label{sec:condemner-implementations}

% \pragmaonce

% adapted from https://www.overleaf.com/learn/latex/Commands
\providecommand{\dissertationelse}[2]{%
% adapted from https://tex.stackexchange.com/a/33577
\ifdefined\DISSERTATION
#1
\else
#2
\fi
}

\provideenvironment{lstinputlistinghandle}{}{}

{\makeatletter\if@twocolumn\onecolumn\fi\makeatother
\begin{lstinputlistinghandle}
\lstinputlisting[%
language=Python,
caption={
  Depth-proportional resolution policy condemner implementation.
},
label={lst:StratumRetentionCondemnerDepthProportionalResolution},
style=mypython,
basicstyle=\dissertationelse{\fontsize{9}{10}\selectfont}{\scriptsize},
]{submodules/hstrat/hstrat/hstrat/stratum_retention_condemners/StratumRetentionCondemnerDepthProportionalResolution.py}
\end{lstinputlistinghandle}
}

\provideenvironment{lstinputlistinghandle}{}{}

{\makeatletter\if@twocolumn\onecolumn\fi\makeatother
\begin{lstinputlistinghandle}
\lstinputlisting[%
language=Python,
caption={
  Fixed resolution policy condemner implementation.
},
label={lst:StratumRetentionCondemnerFixedResolution},
style=mypython,
basicstyle=\dissertationelse{\fontsize{9}{10}\selectfont}{\scriptsize},
]{submodules/hstrat/hstrat/hstrat/stratum_retention_condemners/StratumRetentionCondemnerFixedResolution.py}
\end{lstinputlistinghandle}
}

\provideenvironment{lstinputlistinghandle}{}{}

{\makeatletter\if@twocolumn\onecolumn\fi\makeatother
\begin{lstinputlistinghandle}
\lstinputlisting[%
language=Python,
caption={
  MRCA-recency-proportional resolution policy condemner implementation.
},
label={lst:StratumRetentionCondemnerRecencyProportionalResolution},
style=mypython,
basicstyle=\dissertationelse{\fontsize{9}{10}\selectfont}{\scriptsize},
]{submodules/hstrat/hstrat/hstrat/stratum_retention_condemners/StratumRetentionCondemnerRecencyProportionalResolution.py}
\end{lstinputlistinghandle}
}

\provideenvironment{lstinputlistinghandle}{}{}

{\makeatletter\if@twocolumn\onecolumn\fi\makeatother
\begin{lstinputlistinghandle}
\lstinputlisting[%
language=Python,
caption={
  Tapered depth-proportional resolution policy condemner implementation.
},
label={lst:StratumRetentionCondemnerTaperedDepthProportionalResolution},
style=mypython,
basicstyle=\dissertationelse{\fontsize{9}{10}\selectfont}{\scriptsize},
]{submodules/hstrat/hstrat/hstrat/stratum_retention_condemners/StratumRetentionCondemnerTaperedDepthProportionalResolution.py}
\end{lstinputlistinghandle}
}
