# Supplementary material for: Algorithms for Efficient, Compact Online Data Stream Curation
Source: arXiv:2403.00266 source file (2024-03-01)
Supplement: Supplementary file 9 [file differentia-size-full.tex]

\section{Differentia Size} \label{sec:differentia-size-full}
