# Supplementary material for: Algorithms for Efficient, Compact Online Data Stream Curation
Source: arXiv:2403.00266 source file (2024-03-01)
Supplement: Supplementary file 10 [file memory-footprint-outcomes.tex]

\section{Memory Footprint Outcomes} \label{sec:memory_footprint_outcomes}

% \pragmaonce
% ^adapted from https://tex.stackexchange.com/a/195173

% adapted from https://tex.stackexchange.com/a/118450
\providecommand{
\def\dataname{}\def\fulldataname{}% \input{lib/importpath.tex}
\makeatletter
  \def\importpathx{\import@path}
\makeatother

\begin{table}

\begin{tabularx}{\columnwidth}{X | X | X | X | X | X}%
  \adjustbox{
    minipage=12em,
    rotate=90,
  }{
    \raggedright
    \bfseries
    Target Per-Column Memory Footprint (bits)
    \par
  }
  & \adjustbox{
      minipage=12em,
      rotate=90,
    }{
      \raggedright
      \bfseries
      Actual Mean Per-Column Memory Footprint (bits)
      \par
  }
  & \adjustbox{
      minipage=12em,
      rotate=90,
    }{
      \raggedright
      \bfseries
      Memory Footprint Percent Error
      \par
  }
  & \adjustbox{
      minipage=12em,
      rotate=90,
    }{
      \raggedright
      \bfseries
      Fingerprint Differentia Width (bits)
      \par
  }
  & \adjustbox{
      minipage=12em,
      rotate=90,
    }{
      \raggedright
      \bfseries
      Stratum Retention Policy
      \par
  }
  & \adjustbox{
      minipage=12em,
      rotate=90,
    }{
      \raggedright
      \bfseries
      Retention Policy Resolution Parameter
      \par
  }
  \\\hline\hline  % specify table head
  \csvreader[
    filter expr={
          test{\ifnumgreater{\thecsvinputline}{2}}
    }
  ]{\importpathx submodules/hereditary-stratigraph-concept/binder/phylogenetic-inference/\fulldataname }{}% use head of csv as column names
{
  \csvcolix
  & \num[round-precision=1,round-mode=places]{\csvcolii}
  &
  \ifthenelse{
    \lengthtest{\csuse{csvcolii}pt > \csuse{csvcolix}pt}
    }{\cellcolor{red!25}}{}%

  \num[round-precision=1,round-mode=places]{
    \fpeval{ 100 * \csvcolii / \csvcolix - 100 }
  }
  & \csvcolvi
  &
  \StrDel{\csvcolvii}{a}[\temp]
  \StrDel{\temp}{b}[\temp]
  \StrDel{\temp}{c}[\temp]
  \StrDel{\temp}{d}[\temp]
  \StrDel{\temp}{e}[\temp]
  \StrDel{\temp}{f}[\temp]
  \StrDel{\temp}{g}[\temp]
  \StrDel{\temp}{h}[\temp]
  \StrDel{\temp}{i}[\temp]
  \StrDel{\temp}{j}[\temp]
  \StrDel{\temp}{k}[\temp]
  \StrDel{\temp}{l}[\temp]
  \StrDel{\temp}{m}[\temp]
  \StrDel{\temp}{n}[\temp]
  \StrDel{\temp}{o}[\temp]
  \StrDel{\temp}{p}[\temp]
  \StrDel{\temp}{q}[\temp]
  \StrDel{\temp}{r}[\temp]
  \StrDel{\temp}{s}[\temp]
  \StrDel{\temp}{t}[\temp]
  \StrDel{\temp}{u}[\temp]
  \StrDel{\temp}{v}[\temp]
  \StrDel{\temp}{w}[\temp]
  \StrDel{\temp}{x}[\temp]
  \StrDel{\temp}{y}[\temp]
  \StrDel{\temp}{z}
  & \csvcolviii
  \\
}% specify your columns here
\end{tabularx}
\caption{
Hereditary stratigraph column memory footprint outcomes for phylogenetic reconstruction experiments on the \dataname dataset.
All treatments' stratum retention policies were parameterized to use as much of the target per-column memory footprint as possible without exceeding it.
Treatments where the stratum retention policy could not be parameterized low enough to meet the target per-column memory footprint are highlighted in red.
TDPR denotes the ``Tapered Depth-Proportional Resolution'' policy and RPR denotes the ``Recency-Proportional Resolution'' policy.
}

% adapted from https://tex.stackexchange.com/a/15708
\StrSubstitute{\dataname}{ }{-}[\temp]
\StrSubstitute{\temp}{A}{a}[\temp]
\StrSubstitute{\temp}{B}{b}[\temp]
\StrSubstitute{\temp}{C}{c}[\temp]
\StrSubstitute{\temp}{D}{d}[\temp]
\StrSubstitute{\temp}{E}{e}[\temp]
\StrSubstitute{\temp}{F}{f}[\temp]
\StrSubstitute{\temp}{G}{g}[\temp]
\StrSubstitute{\temp}{H}{h}[\temp]
\StrSubstitute{\temp}{I}{i}[\temp]
\StrSubstitute{\temp}{J}{j}[\temp]
\StrSubstitute{\temp}{K}{k}[\temp]
\StrSubstitute{\temp}{L}{l}[\temp]
\StrSubstitute{\temp}{M}{m}[\temp]
\StrSubstitute{\temp}{N}{n}[\temp]
\StrSubstitute{\temp}{O}{o}[\temp]
\StrSubstitute{\temp}{P}{p}[\temp]
\StrSubstitute{\temp}{Q}{q}[\temp]
\StrSubstitute{\temp}{R}{r}[\temp]
\StrSubstitute{\temp}{S}{s}[\temp]
\StrSubstitute{\temp}{T}{t}[\temp]
\StrSubstitute{\temp}{U}{u}[\temp]
\StrSubstitute{\temp}{V}{v}[\temp]
\StrSubstitute{\temp}{w}{w}[\temp]
\StrSubstitute{\temp}{X}{x}[\temp]
\StrSubstitute{\temp}{Y}{y}[\temp]
\StrSubstitute{\temp}{Z}{z}[\temp]

\def\labeltext{%
  {tab:experiment-column-sizes-\temp}%
}
\expandafter\label\labeltext
\end{table}

}[2]{
\def\dataname{#1}\def\fulldataname{#2}% \input{lib/importpath.tex}
\makeatletter
  \def\importpathx{\import@path}
\makeatother

\begin{table}

\begin{tabularx}{\columnwidth}{X | X | X | X | X | X}%
  \adjustbox{
    minipage=12em,
    rotate=90,
  }{
    \raggedright
    \bfseries
    Target Per-Column Memory Footprint (bits)
    \par
  }
  & \adjustbox{
      minipage=12em,
      rotate=90,
    }{
      \raggedright
      \bfseries
      Actual Mean Per-Column Memory Footprint (bits)
      \par
  }
  & \adjustbox{
      minipage=12em,
      rotate=90,
    }{
      \raggedright
      \bfseries
      Memory Footprint Percent Error
      \par
  }
  & \adjustbox{
      minipage=12em,
      rotate=90,
    }{
      \raggedright
      \bfseries
      Fingerprint Differentia Width (bits)
      \par
  }
  & \adjustbox{
      minipage=12em,
      rotate=90,
    }{
      \raggedright
      \bfseries
      Stratum Retention Policy
      \par
  }
  & \adjustbox{
      minipage=12em,
      rotate=90,
    }{
      \raggedright
      \bfseries
      Retention Policy Resolution Parameter
      \par
  }
  \\\hline\hline  % specify table head
  \csvreader[
    filter expr={
          test{\ifnumgreater{\thecsvinputline}{2}}
    }
  ]{\importpathx submodules/hereditary-stratigraph-concept/binder/phylogenetic-inference/\fulldataname }{}% use head of csv as column names
{
  \csvcolix
  & \num[round-precision=1,round-mode=places]{\csvcolii}
  &
  \ifthenelse{
    \lengthtest{\csuse{csvcolii}pt > \csuse{csvcolix}pt}
    }{\cellcolor{red!25}}{}%

  \num[round-precision=1,round-mode=places]{
    \fpeval{ 100 * \csvcolii / \csvcolix - 100 }
  }
  & \csvcolvi
  &
  \StrDel{\csvcolvii}{a}[\temp]
  \StrDel{\temp}{b}[\temp]
  \StrDel{\temp}{c}[\temp]
  \StrDel{\temp}{d}[\temp]
  \StrDel{\temp}{e}[\temp]
  \StrDel{\temp}{f}[\temp]
  \StrDel{\temp}{g}[\temp]
  \StrDel{\temp}{h}[\temp]
  \StrDel{\temp}{i}[\temp]
  \StrDel{\temp}{j}[\temp]
  \StrDel{\temp}{k}[\temp]
  \StrDel{\temp}{l}[\temp]
  \StrDel{\temp}{m}[\temp]
  \StrDel{\temp}{n}[\temp]
  \StrDel{\temp}{o}[\temp]
  \StrDel{\temp}{p}[\temp]
  \StrDel{\temp}{q}[\temp]
  \StrDel{\temp}{r}[\temp]
  \StrDel{\temp}{s}[\temp]
  \StrDel{\temp}{t}[\temp]
  \StrDel{\temp}{u}[\temp]
  \StrDel{\temp}{v}[\temp]
  \StrDel{\temp}{w}[\temp]
  \StrDel{\temp}{x}[\temp]
  \StrDel{\temp}{y}[\temp]
  \StrDel{\temp}{z}
  & \csvcolviii
  \\
}% specify your columns here
\end{tabularx}
\caption{
Hereditary stratigraph column memory footprint outcomes for phylogenetic reconstruction experiments on the \dataname dataset.
All treatments' stratum retention policies were parameterized to use as much of the target per-column memory footprint as possible without exceeding it.
Treatments where the stratum retention policy could not be parameterized low enough to meet the target per-column memory footprint are highlighted in red.
TDPR denotes the ``Tapered Depth-Proportional Resolution'' policy and RPR denotes the ``Recency-Proportional Resolution'' policy.
}

% adapted from https://tex.stackexchange.com/a/15708
\StrSubstitute{\dataname}{ }{-}[\temp]
\StrSubstitute{\temp}{A}{a}[\temp]
\StrSubstitute{\temp}{B}{b}[\temp]
\StrSubstitute{\temp}{C}{c}[\temp]
\StrSubstitute{\temp}{D}{d}[\temp]
\StrSubstitute{\temp}{E}{e}[\temp]
\StrSubstitute{\temp}{F}{f}[\temp]
\StrSubstitute{\temp}{G}{g}[\temp]
\StrSubstitute{\temp}{H}{h}[\temp]
\StrSubstitute{\temp}{I}{i}[\temp]
\StrSubstitute{\temp}{J}{j}[\temp]
\StrSubstitute{\temp}{K}{k}[\temp]
\StrSubstitute{\temp}{L}{l}[\temp]
\StrSubstitute{\temp}{M}{m}[\temp]
\StrSubstitute{\temp}{N}{n}[\temp]
\StrSubstitute{\temp}{O}{o}[\temp]
\StrSubstitute{\temp}{P}{p}[\temp]
\StrSubstitute{\temp}{Q}{q}[\temp]
\StrSubstitute{\temp}{R}{r}[\temp]
\StrSubstitute{\temp}{S}{s}[\temp]
\StrSubstitute{\temp}{T}{t}[\temp]
\StrSubstitute{\temp}{U}{u}[\temp]
\StrSubstitute{\temp}{V}{v}[\temp]
\StrSubstitute{\temp}{w}{w}[\temp]
\StrSubstitute{\temp}{X}{x}[\temp]
\StrSubstitute{\temp}{Y}{y}[\temp]
\StrSubstitute{\temp}{Z}{z}[\temp]

\def\labeltext{%
  {tab:experiment-column-sizes-\temp}%
}
\expandafter\label\labeltext
\end{table}

}

\def\dataname{NK EcoEA Selection}\def\fulldataname{a=actual_retained_bits+source=nk_ecoeaselection_seed110_pop100_mut.01_snapshot_3000.csv}

\def\dataname{NK Lexicase Selection}\def\fulldataname{a=actual_retained_bits+source=nk_lexicaseselection_seed110_pop165_mut.01_snapshot_500.csv}

\def\dataname{NK Random Selection}\def\fulldataname{a=actual_retained_bits+source=nk_randomselection_seed7_pop100_mut.01_snapshot_5000.csv}

\def\dataname{NK Sharing Selection}\def\fulldataname{a=actual_retained_bits+source=nk_sharingselection_seed10_pop100_mut.01_snapshot_5000.csv}

\def\dataname{NK Tournament Selection}\def\fulldataname{a=actual_retained_bits+source=nk_tournamentselection_seed140_pop100_mut.01_snapshot_5000.csv}
