# Supplementary material for: Algorithms for Efficient, Compact Online Data Stream Curation
Source: arXiv:2403.00266 source file (2024-03-01)
Supplement: Supplementary file 11 [file miscellaneous.tex]

\section{Miscellaneous} \label{sec:hstrat-miscellaneous}

\begin{sidewaystable}[]
\begin{tabular}{lllll}
Selection Scheme & Per-bit Mutation Rate & Number Generations & Population Size & Phylogeny Download URL \\
Eco-EA           & 0.01                  & 3000               & 100             & \url{https://osf.io/5d3be/} \\
Lexicase         & 0.01                  & 500                & 165             & \url{https://osf.io/8ycq7/} \\
Random           & 0.01                  & 5000               & 100             & \url{https://osf.io/ydxt7/} \\
Sharing          & 0.01                  & 5000               & 100             & \url{https://osf.io/cz9fk/} \\
Tournament       & 0.01                  & 5000               & 100             & \url{https://osf.io/5ubn8/}
\end{tabular}
\caption{
Evolutionary conditions of ground-truth phylogenies taken from \citep{dolson2018applying}.
} \label{tab:ground-truth-phylogenies}
\end{sidewaystable}
