# Supplementary material for: Algorithms for Efficient, Compact Online Data Stream Curation
Source: arXiv:2403.00266 source file (2024-03-01)
Supplement: Supplementary file 12 [file predicate-implementations.tex]

\section{Predicate Implementations}
\label{sec:predicate-implementations}

\provideenvironment{lstinputlistinghandle}{}{}

{\makeatletter\if@twocolumn\onecolumn\fi\makeatother
\begin{lstinputlistinghandle}
\lstinputlisting[%
language=Python,
caption={
  Depth-proportional resolution policy predicate implementation, including method to calculate exact number of strata retained by generation and method to calculate stratum deposition rank from column index.
},
label={lst:StratumRetentionPredicateDepthProportionalResolution},
style=mypython,
basicstyle=\dissertationelse{\fontsize{9}{10}\selectfont}{\scriptsize},
]{submodules/hstrat/hstrat/hstrat/stratum_retention_predicates/StratumRetentionPredicateDepthProportionalResolution.py}
\end{lstinputlistinghandle}
}

\provideenvironment{lstinputlistinghandle}{}{}

{\makeatletter\if@twocolumn\onecolumn\fi\makeatother
\begin{lstinputlistinghandle}
\lstinputlisting[%
language=Python,
caption={
  Fixed resolution policy predicate implementation, including method to calculate exact number of strata retained by generation and method to calculate stratum deposition rank from column index.
},
label={lst:StratumRetentionPredicateFixedResolution},
style=mypython,
basicstyle=\dissertationelse{\fontsize{9}{10}\selectfont}{\scriptsize},
]{submodules/hstrat/hstrat/hstrat/stratum_retention_predicates/StratumRetentionPredicateFixedResolution.py}
\end{lstinputlistinghandle}
}

\provideenvironment{lstinputlistinghandle}{}{}

{\makeatletter\if@twocolumn\onecolumn\fi\makeatother
\begin{lstinputlistinghandle}
\lstinputlisting[%
language=Python,
caption={
  MRCA-recency-proportional resolution policy predicate implementation, including method to calculate exact number of strata retained by generation and method to calculate stratum deposition rank from column index.
},
label={lst:StratumRetentionPredicateRecencyProportionalResolution},
style=mypython,
basicstyle=\dissertationelse{\fontsize{9}{10}\selectfont}{\scriptsize},
]{submodules/hstrat/hstrat/hstrat/stratum_retention_predicates/StratumRetentionPredicateRecencyProportionalResolution.py}
\end{lstinputlistinghandle}
}

\provideenvironment{lstinputlistinghandle}{}{}

{\makeatletter\if@twocolumn\onecolumn\fi\makeatother
\begin{lstinputlistinghandle}
\lstinputlisting[%
language=Python,
caption={
  Tapered depth-proportional resolution policy predicate implementation, including method to calculate exact number of strata retained by generation and method to calculate stratum deposition rank from column index.
},
label={lst:StratumRetentionPredicateTaperedDepthProportionalResolution},
style=mypython,
basicstyle=\dissertationelse{\fontsize{9}{10}\selectfont}{\scriptsize},
]{submodules/hstrat/hstrat/hstrat/stratum_retention_predicates/StratumRetentionPredicateTaperedDepthProportionalResolution.py}
\end{lstinputlistinghandle}
}
