# Supplementary material for: Algorithms for Efficient, Compact Online Data Stream Curation
Source: arXiv:2403.00266 source file (2024-03-01)
Supplement: Supplementary file 13 [file retention-policy-full.tex]

\section{Retention Policy} \label{sec:retention-policy-full}
