# Supplementary material for: Algorithms for Efficient, Compact Online Data Stream Curation
Source: arXiv:2403.00266 source file (2024-03-01)
Supplement: Supplementary file 20 [file retention-policy-full.tex]

{
\onecolumn
\section{Retention Policy} \label{sec:retention-policy-full}

\csvreader[
  longtable=cccccc,
  table head=\caption{
    Comparison of phylogenetic reconstruction quality between stratum retention policies.
    Reconstruction quality measured as clustering information distance (lower is better), mutual clustering information (higher is better), and generalized Robinson-Foulds similarity (higher is better) between reconstructed phylogeny and ground truth phylogeny \citep{smith2020information, smith2020treedist}.  }\label{tab:reconstruction-quality-results-by-policy} \\
    \toprule \thead{Tree Comparison Metric} & \thead{Selection\\ Scheme} & \thead{Num\\ Differentia\\ Bits} & \thead{Target\\ Num\\ Column\\ Bits} & \thead{Recency- \\Proportional \\ Resolution\\ Score} & \thead{Tapered\\ Depth-\\ Proportional\\ Resolution\\ Score} \\ \midrule\endhead
    \bottomrule\endfoot,
  late after line=\\,
]{%
submodules/hereditary-stratigraph-concept/binder/reconstruction-quality/outplots/reconstruction_quality_results_by_policy.csv%
}{}{%
\csvcoli & \csvcolii & \csvcoliii & \csvcoliv & \csvcolv & \csvcolvi
}

\begin{figure*}
    \includegraphics[width=\linewidth]{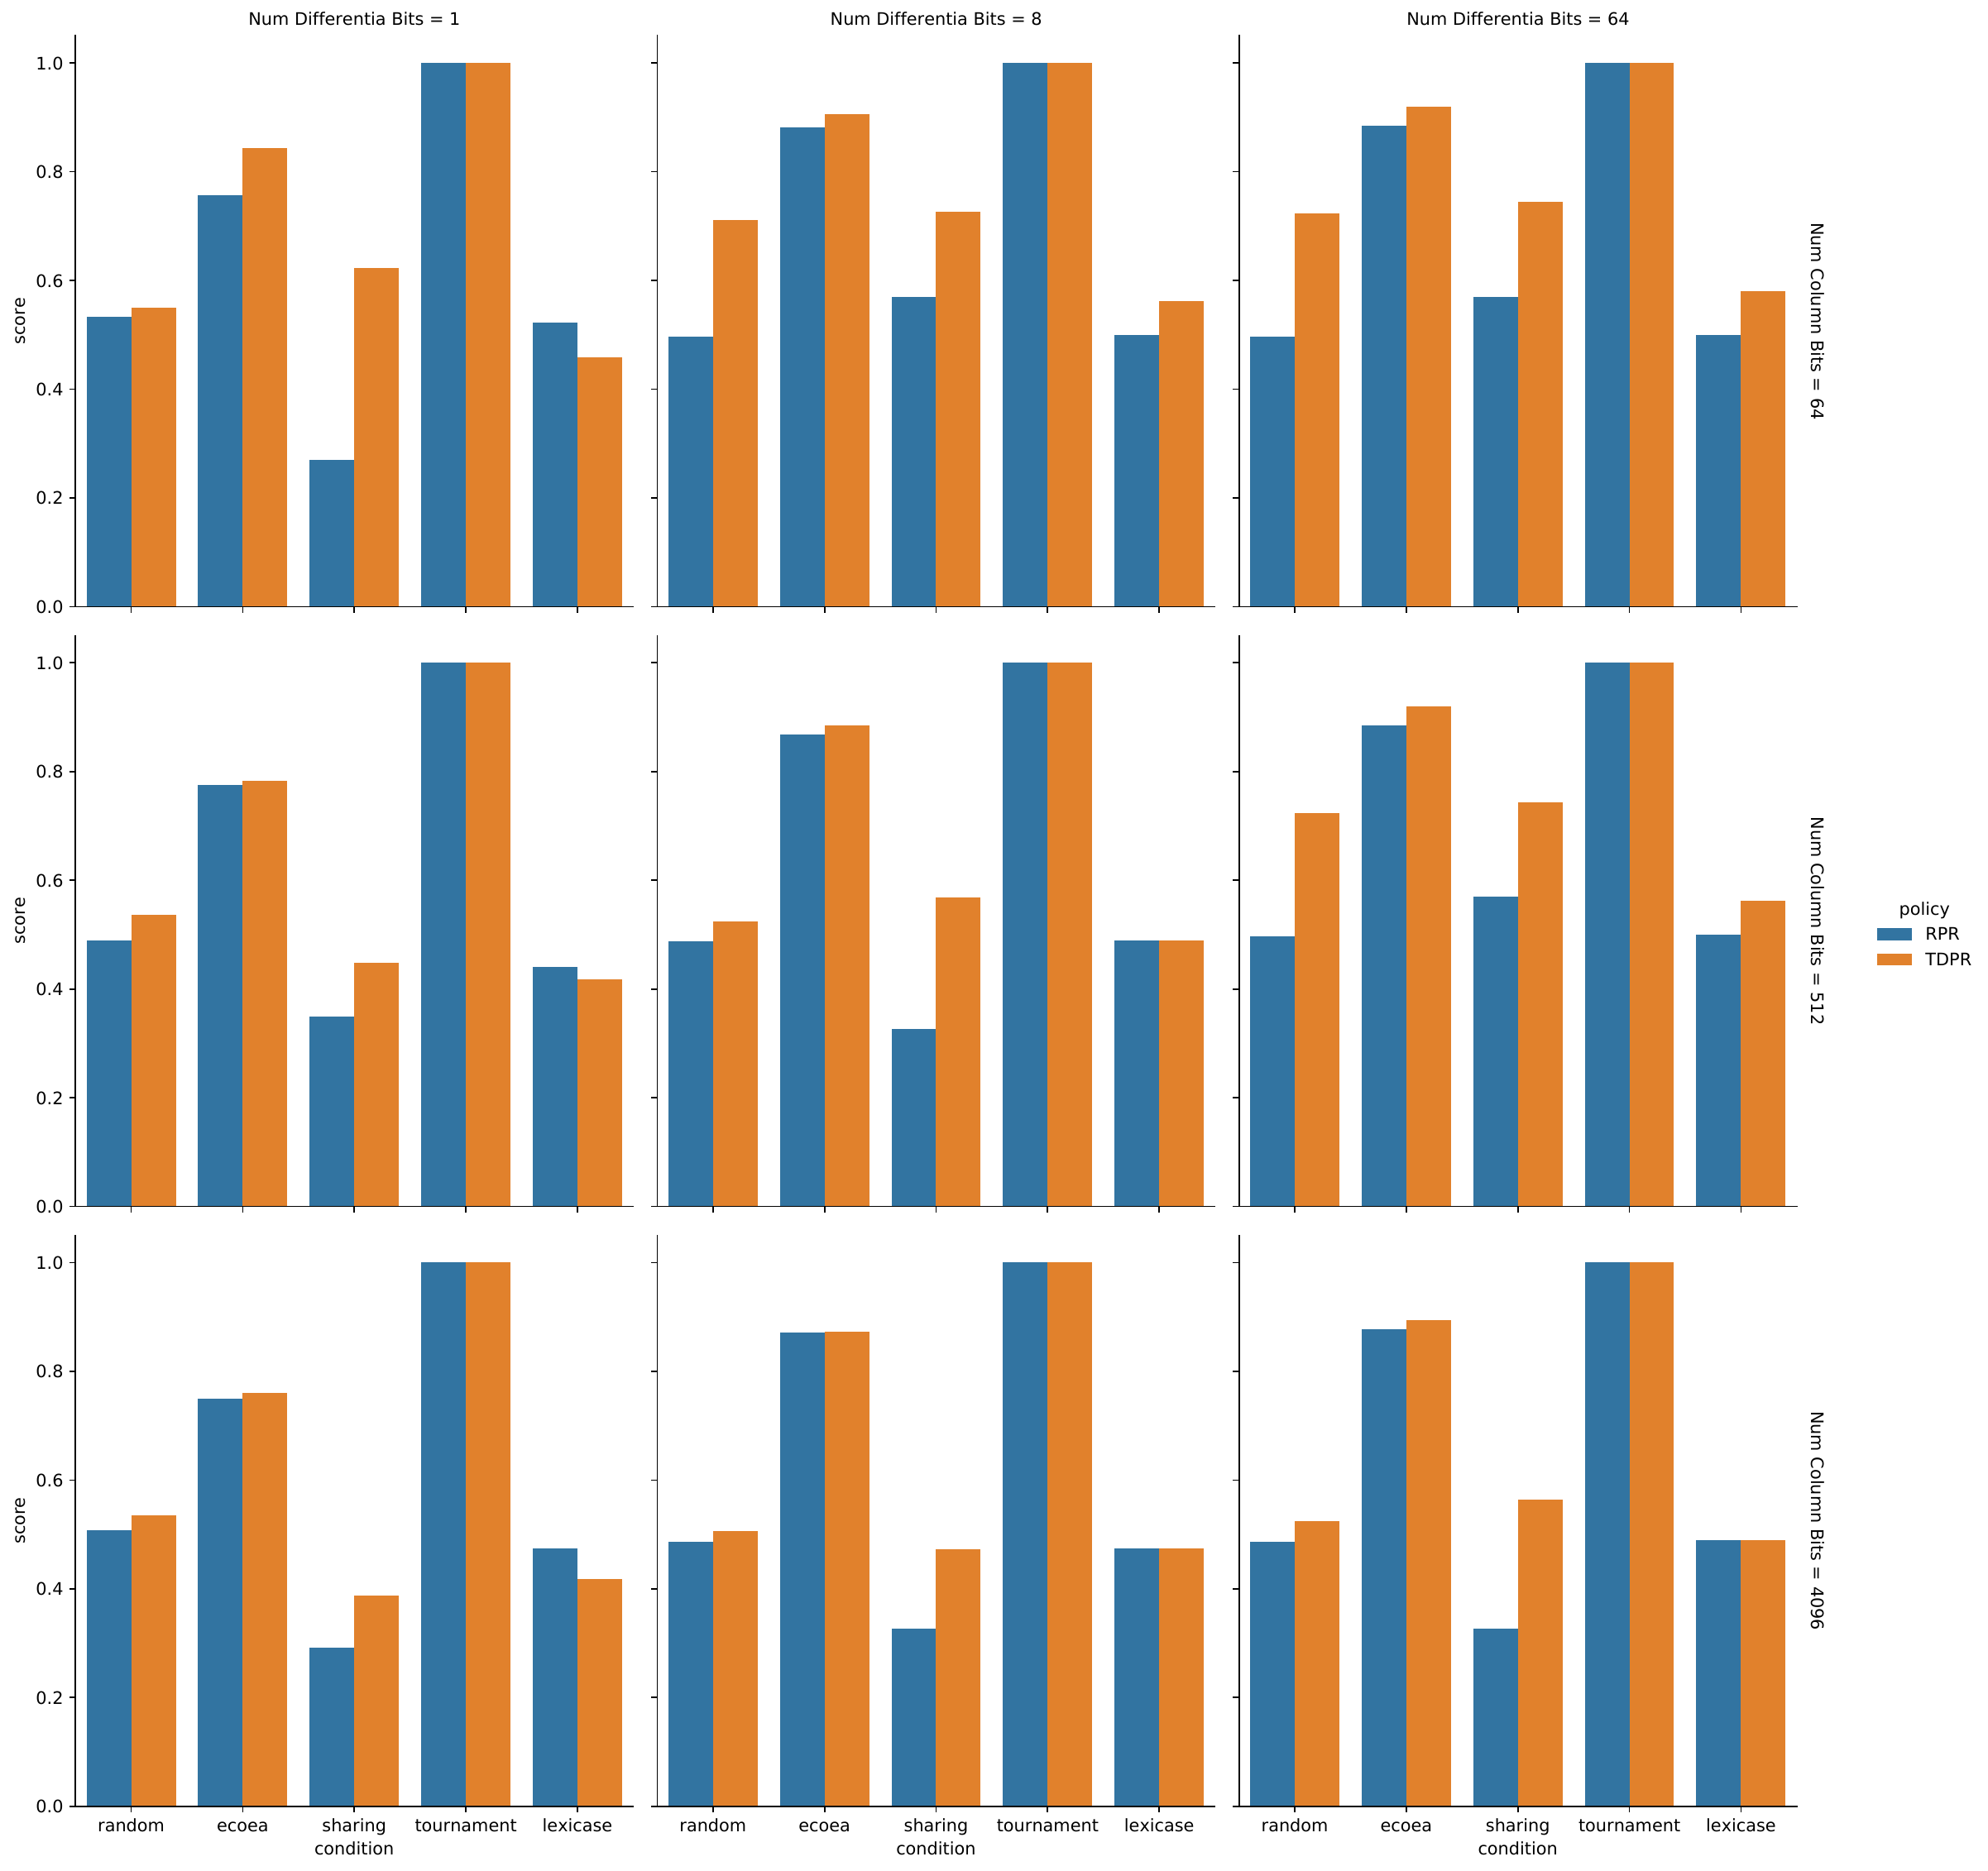}
    \caption{
    Comparison of phylogenetic reconstruction quality between stratum retention policies.
    Reconstruction quality measured as clustering information distance between reconstructed phylogeny and ground truth phylogeny \citep{smith2020information, smith2020treedist}.
    Lower is better.
    RPR is recency-proportional resolution stratum retention policy and TDPR is tapered depth-proportional resolution stratum retention policy.
    }
    \label{fig:policy-clustering-information-distance}
\end{figure*}

\begin{figure*}
    \includegraphics[width=\linewidth]{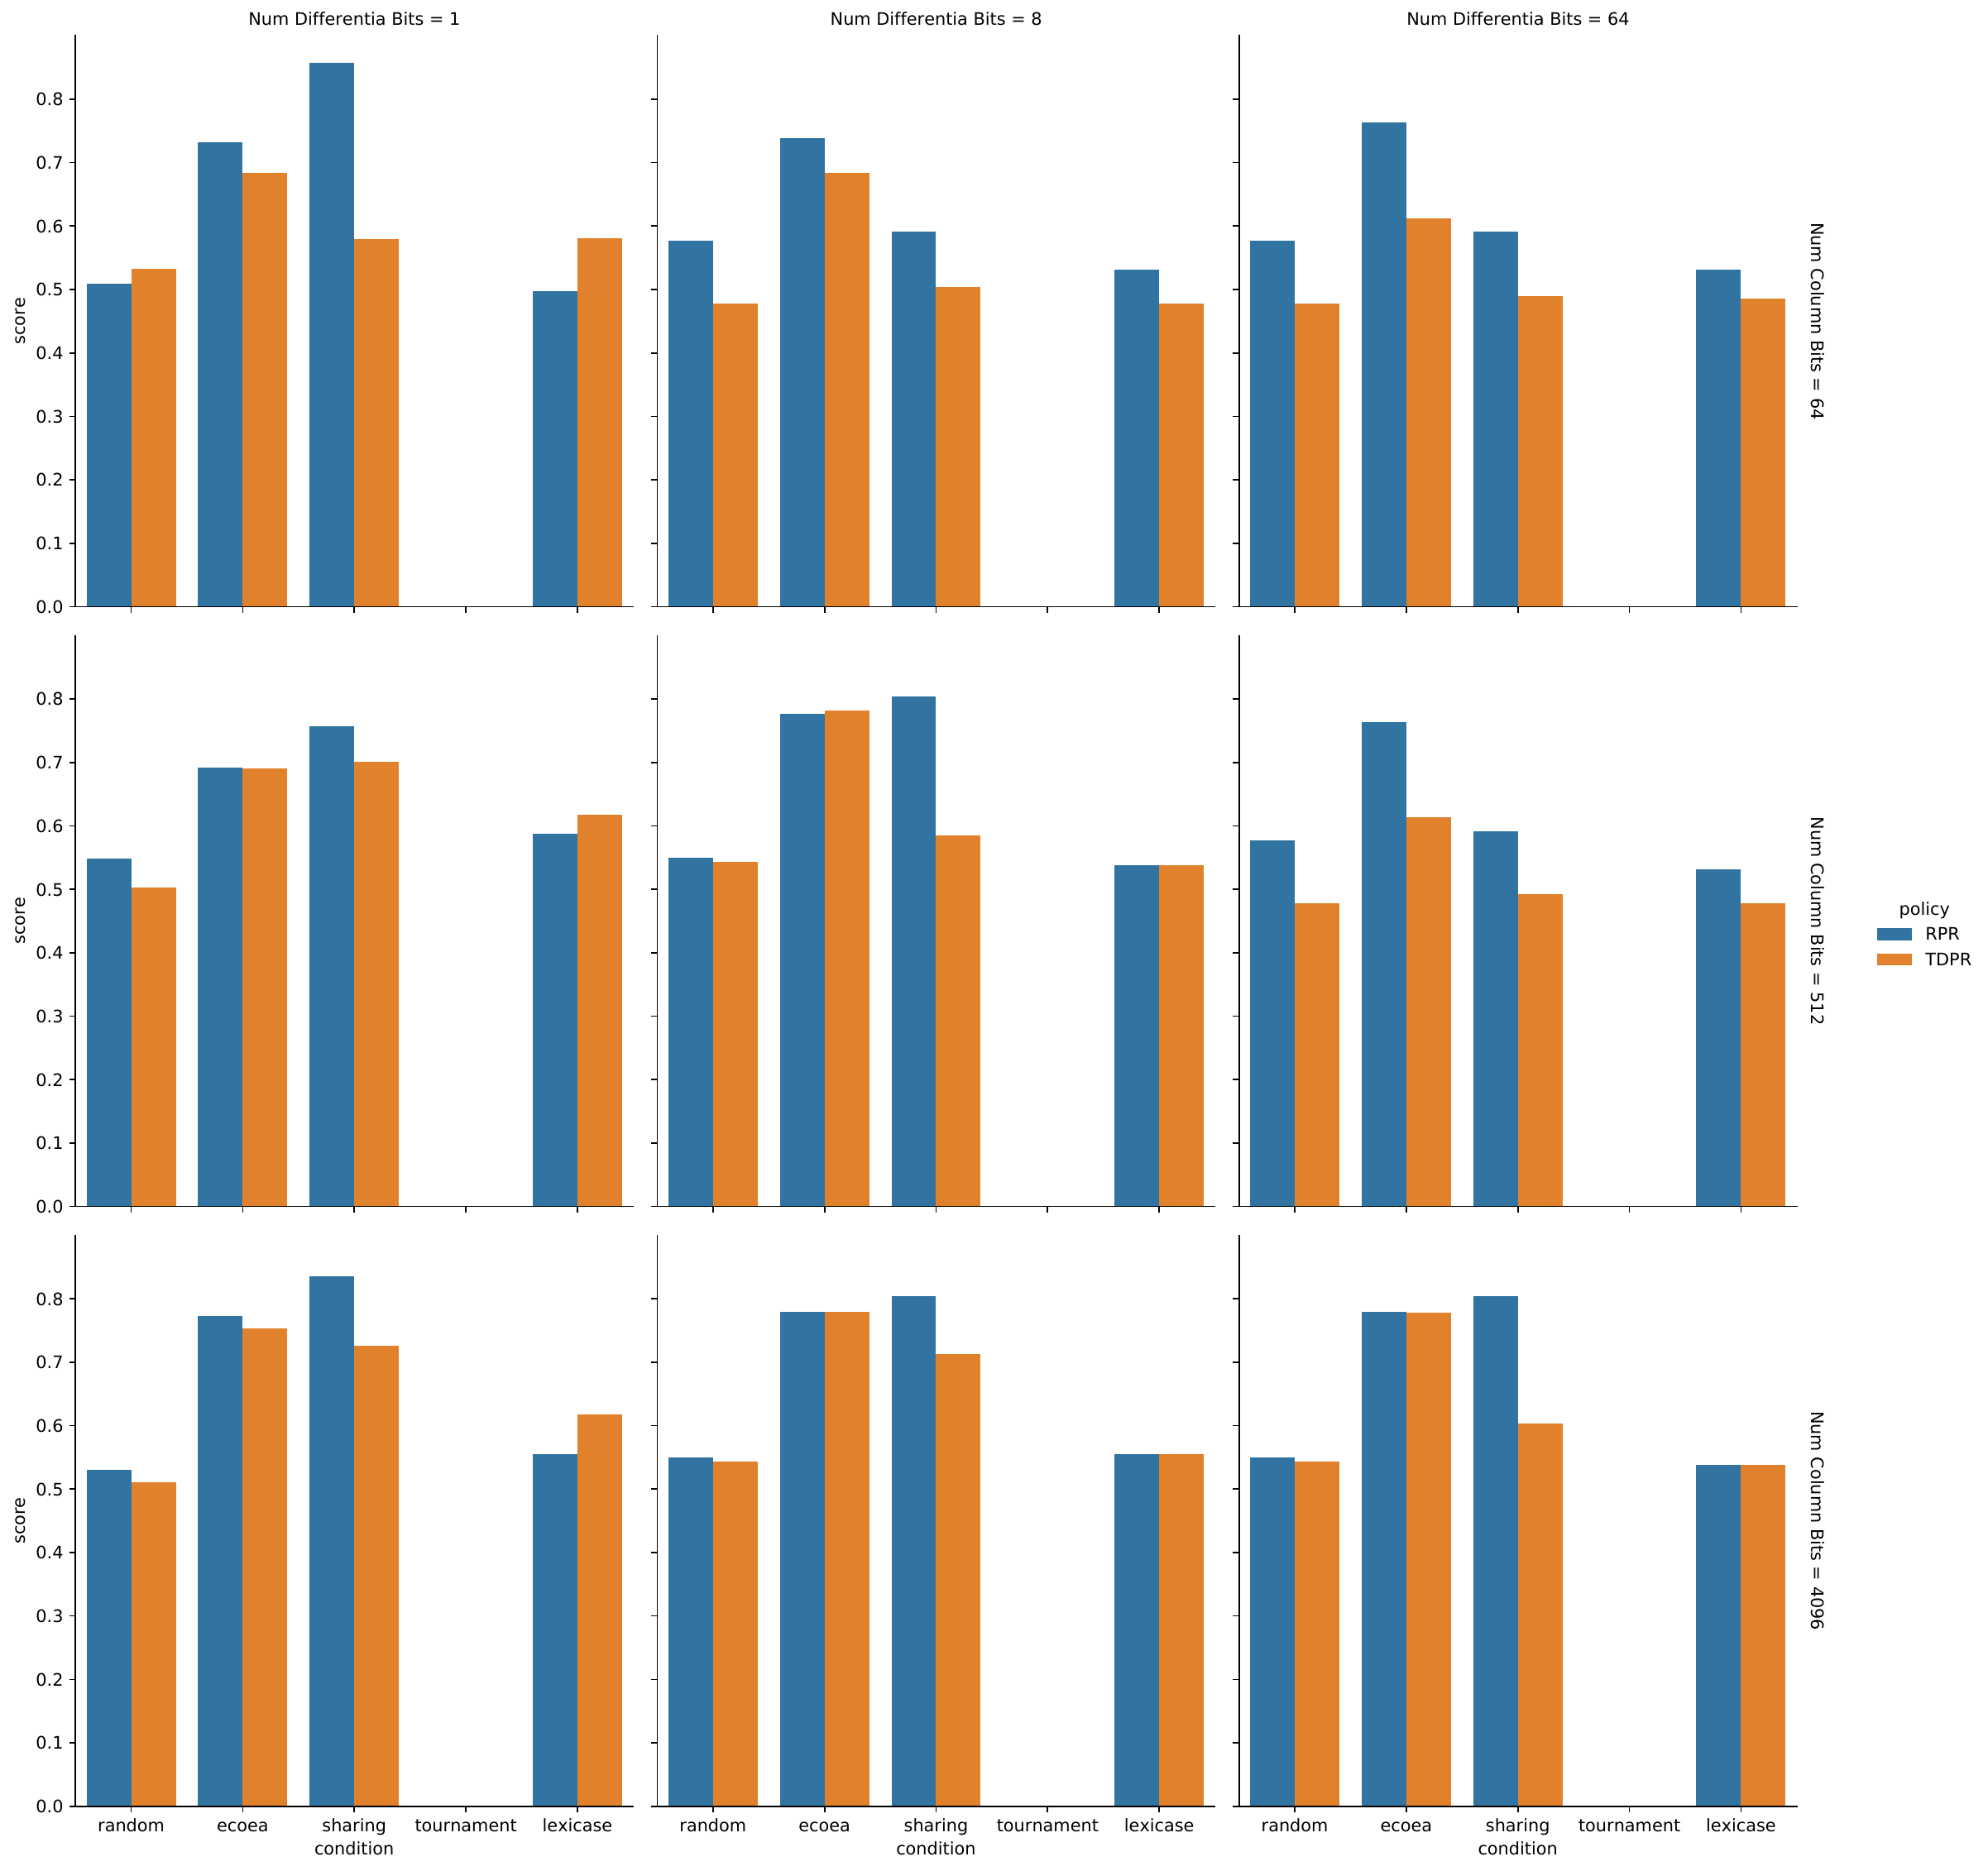}
    \caption{
    Comparison of phylogenetic reconstruction quality between stratum retention policies.
    Reconstruction quality measured as mutual clustering information between reconstructed phylogeny and ground truth phylogeny \citep{smith2020information, smith2020treedist}.
    Higher is better.
    RPR is recency-proportional resolution stratum retention policy and TDPR is tapered depth-proportional resolution stratum retention policy.
    }
    \label{fig:policy-mutual-clustering-information}
\end{figure*}

\begin{figure*}
    \includegraphics[width=\linewidth]{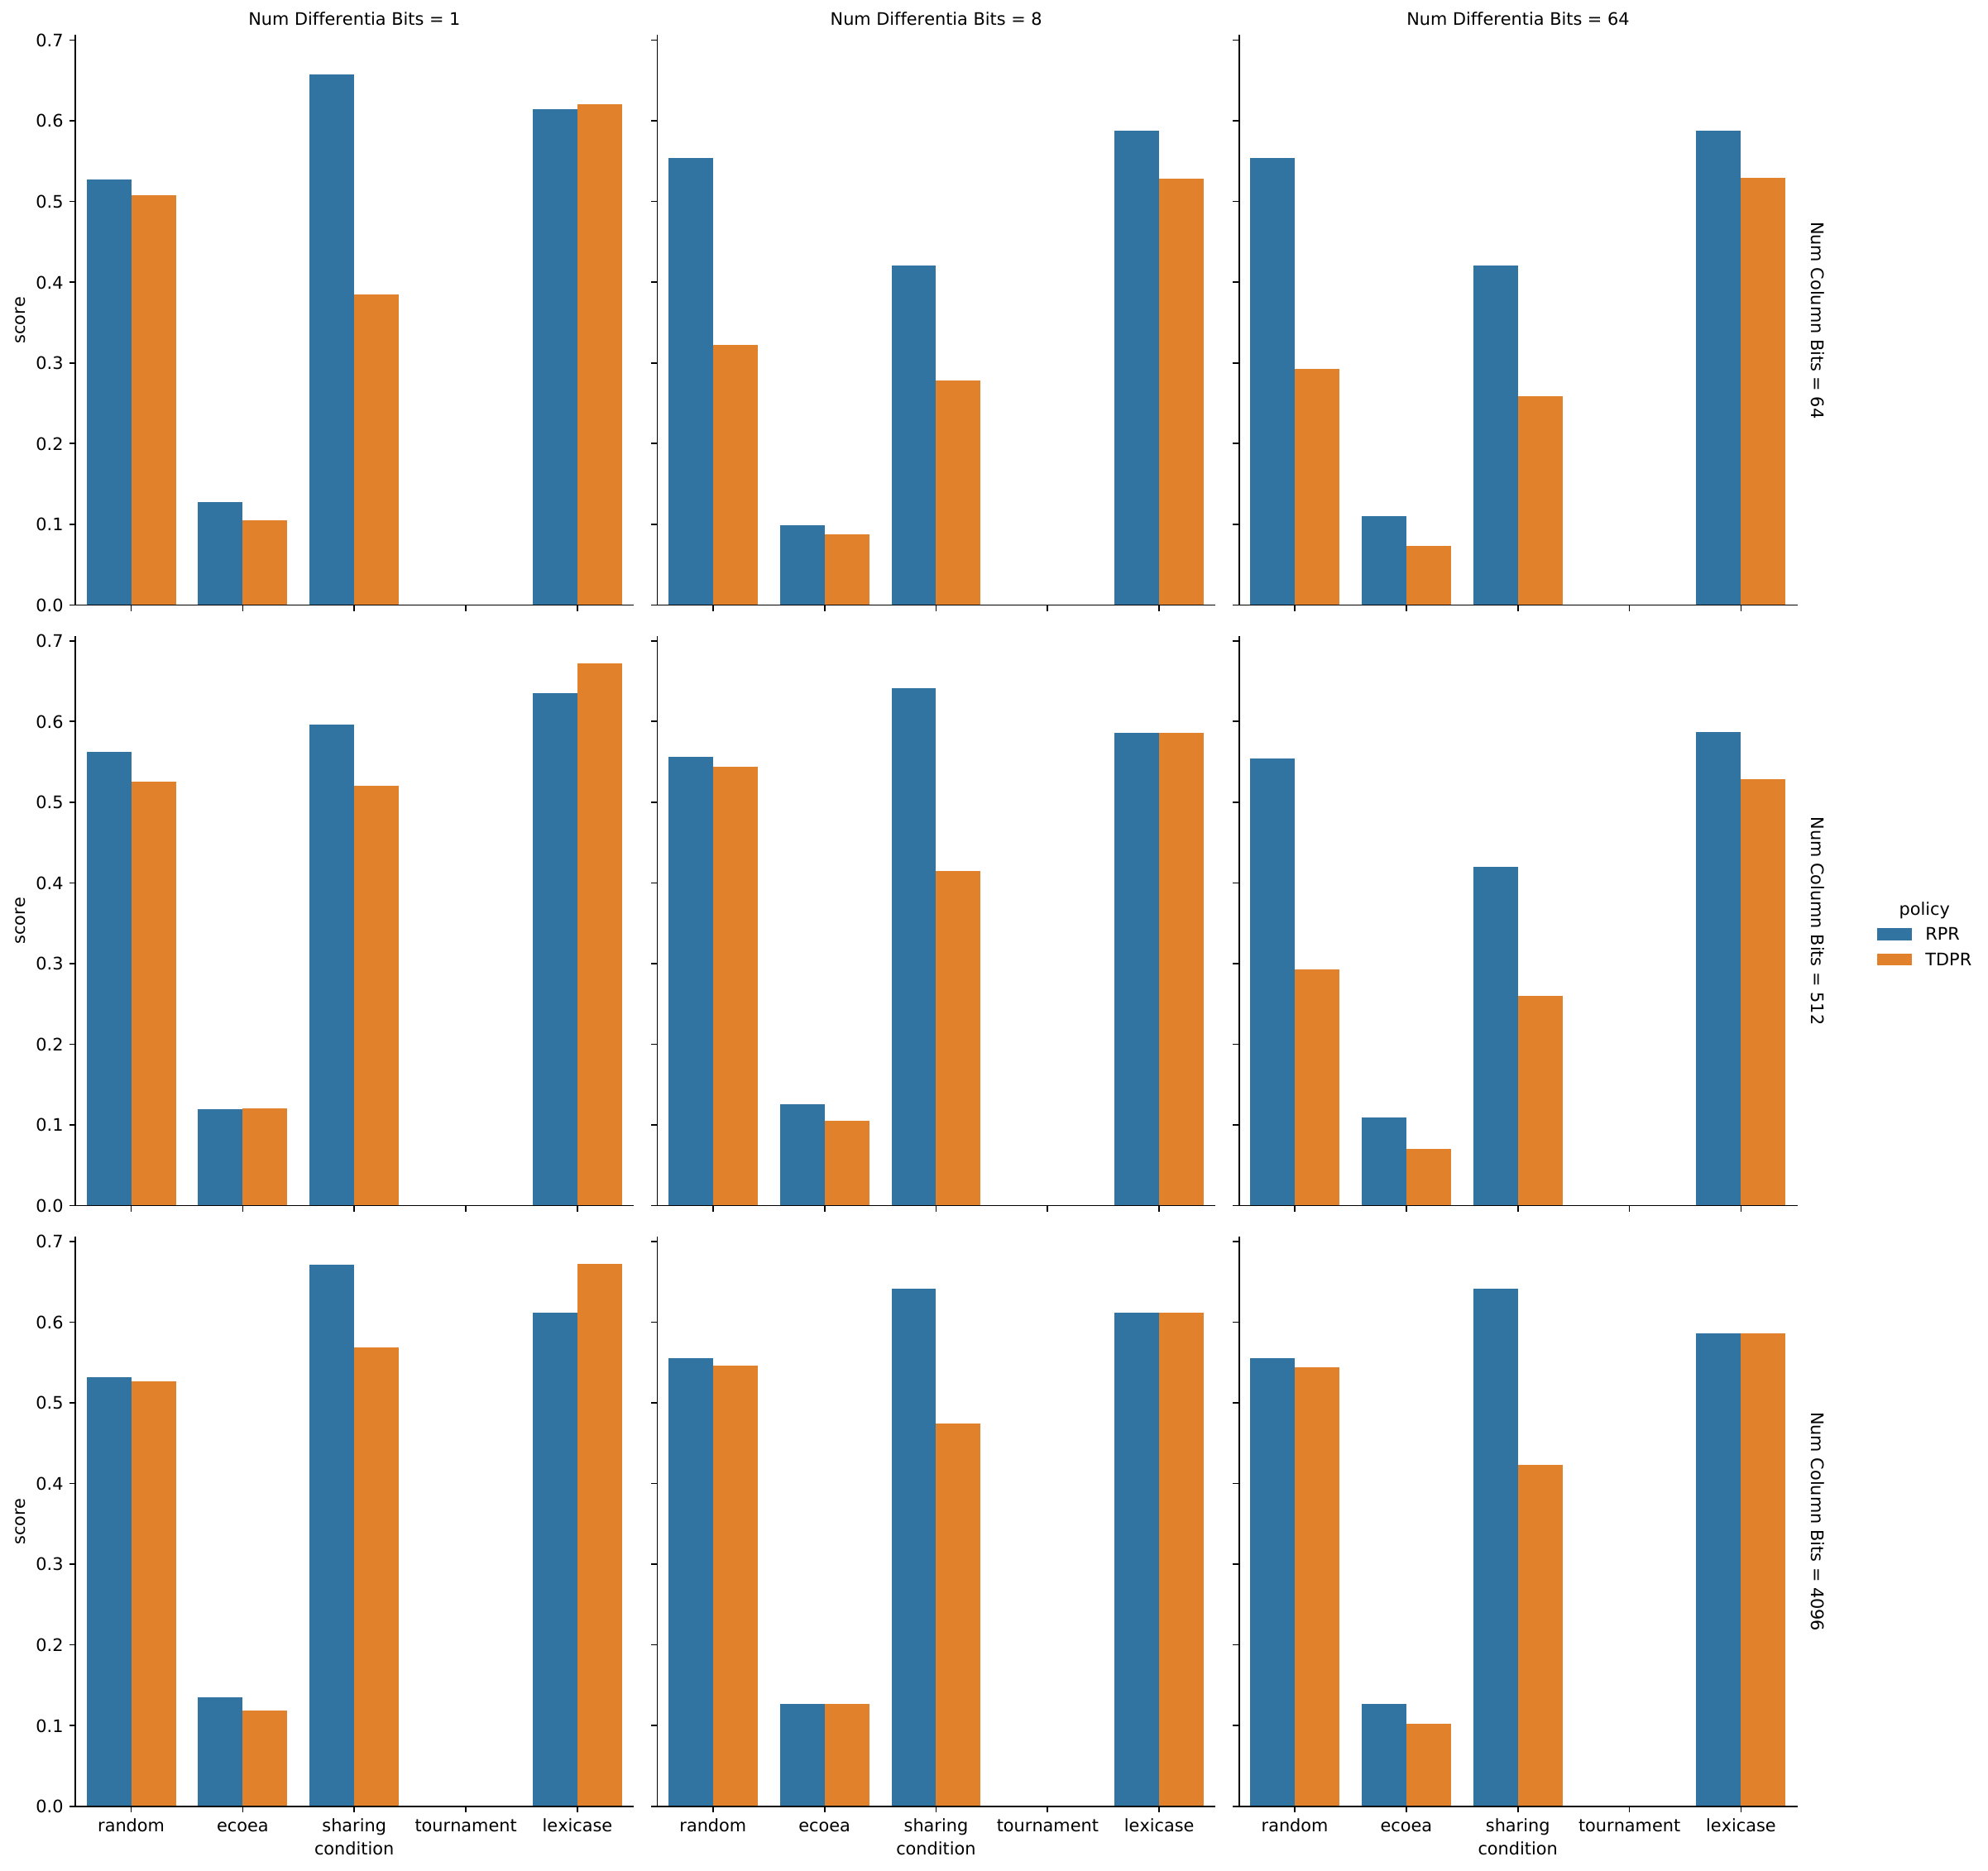}
    \caption{
    Comparison of phylogenetic reconstruction quality between stratum retention policies.
    Reconstruction quality measured as generalized Robinson-Foulds similarity between reconstructed phylogeny and ground truth phylogeny \citep{smith2020information, smith2020treedist}.
    Higher is better.
    RPR is recency-proportional resolution stratum retention policy and TDPR is tapered depth-proportional resolution stratum retention policy.    }
    \label{fig:policy-robinson-foulds-similarity}
\end{figure*}

}
